# Supplementary material for: Auditing Frozen-Encoder Anomaly Detection Across Mechanical Systems: Representation Provenance, Calibration, and Protocol Effects
Source: arXiv:2601.11415 source file (2026-09-01)
Supplement: Supplementary file 1 [file supplemental.tex]

\documentclass[
  aps,
  prapplied,
  onecolumn,
  superscriptaddress
]{revtex4-2}

\usepackage{amsmath}
\usepackage{amssymb}
\usepackage{graphicx}
\usepackage{hyperref}

\begin{document}

\title{Supplemental Material for\\
Zero-Shot Detection of Elastic Transient Morphology Across Physical Systems}

\author{Jose Sánchez Andreu}
\affiliation{Independent Researcher, Murcia, Spain}

\date{\today}

\maketitle

\section{Implementation and Reproducibility Details}
\label{sec:supp_impl}
The purpose of this Supplemental Material is to ensure computational
reproducibility of all reported results while protecting proprietary
representations and training data.

\paragraph{Latent operator.}
The frozen operator $\mathcal{F}$ is implemented as an EfficientNet-B0
convolutional encoder using the \texttt{torchvision} library. The encoder weights are trained on interferometric strain transients only. \cite{tan2019efficientnet}.
The classifier head used during source-domain training maps the pooled
1280-dimensional representation to six interferometric glitch classes and is
discarded for all target-domain experiments.
All results reported in this manuscript are obtained exclusively from the
1280-dimensional latent embeddings produced by the frozen encoder.

\paragraph{Training (source domain only).}
The operator $\mathcal{F}$ is trained only on interferometric strain transients (source domain) using standard supervised optimization with Adam and focal loss to address class imbalance. No target-domain data, labels, or statistics are used at any stage. The final encoder checkpoint is frozen and used without modification in all target-domain experiments.

\paragraph{Time--frequency preprocessing and zero-shot protocol.}
All domains are processed with the same STFT and per-window standardization pipeline (see main text, Sec.~II.C). The encoder is trained once on interferometric transients
and applied zero-shot to all target domains without any adaptation.

\paragraph{Reference distribution and anomaly score.}
A nominal reference distribution $\mathcal{P}_0$ is constructed exclusively
from target-domain data assumed to be nominal (early-life segments in IMS;
normal-state segments in static benchmarks).
Let $\mu$ and $\Sigma$ denote the mean and covariance of the corresponding latent
embeddings.
The window-level anomaly score is defined as the Mahalanobis distance
\[
\mathcal{S}(z)=\sqrt{(z-\mu)^{\top}\Sigma^{-1}(z-\mu)}.
\]
All thresholds, tail statistics, and confidence intervals are computed using
only $\mathcal{P}_0$.
Abnormal windows are never used to estimate $\mu$, $\Sigma$, or the detection
threshold $\tau$.

\section{Public Reproducibility Resources}
\label{sec:supp_repo}

Figure-level reproducibility for all reported plots and numerical values is
provided through derived, non-invertible artifacts, including window-level
anomaly scores, record-level aggregates, thresholds, and bootstrap resamples,
together with deterministic scripts that regenerate each figure from these
artifacts.

For each figure, the public repository includes (i) a data manifest listing all
released artifacts with checksums, and (ii) a single entry-point script that
reproduces the corresponding figure and prints the scalar values reported in
the main text. This release enables independent verification of all reported
drift statistics, AUC values, tail exceedance rates, and confidence intervals,
without requiring access to model weights or source-domain training data.
Our goal is not to claim superiority over optimized, domain-specific condition-monitoring pipelines (e.g., envelope analysis, spectral-kurtosis-based detectors, or supervised diagnostic models tuned to a given machine). Instead, we ask a different question: whether a \emph{single frozen representation}, learned in a distinct precision-physics context, can function as a transferable morphology-sensitive operator under a strict no-adaptation protocol.
For the IMS controlled-split experiments (see the IMS controlled-split protocol in the main text), we additionally
release record-level aggregates ($s_{0.95}$), thresholds $\tau$, tail exceedance counts, and the
RMS/kurtosis descriptors for both the interferometric operator and the ImageNet baseline, together
with deterministic scripts that reproduce the corresponding IMS benchmark tables reported in the main text.
Accordingly, all hyperparameters defining the preprocessing grid and scoring rule are fixed \emph{a priori} and are not selected to maximize performance on any particular target dataset.
Raw sensor data are publicly available from the original dataset providers
(IMS-NASA, CWRU, and VSB) and are not redistributed in this repository.

\begin{center}
\texttt{https://github.com/joseandreuu/aether-morphology-paper}
\end{center}

\section{Training of the Interferometric Operator}
\label{sec:supp_training}

This section specifies the source-domain training of the frozen latent operator $\mathcal{F}$ used throughout the manuscript, while keeping the main text focused on the zero-shot protocol.

\subsection{Training data}
$\mathcal{F}$ is trained on $\sim 1.2\times10^{4}$ labeled interferometric strain-transient events spanning six morphology classes (e.g., blip-like, scattered-light-like, and narrowband whistle-like structures). No target-domain data are used during training.

\subsection{Architecture and embedding}
$\mathcal{F}$ is implemented as an EfficientNet-B0 convolutional encoder.
The classifier head used during source-domain supervision is discarded after training.
All target-domain experiments use only the pooled latent embedding
$z\in\mathbb{R}^{1280}$ produced by the frozen encoder.

\subsection{Optimization}
Training is performed using standard supervised optimization with Adam and focal loss
to mitigate class imbalance. Hyperparameters and training schedules are fixed prior to
target-domain evaluation and do not affect any result reported in this work, as the
encoder is frozen for all zero-shot experiments.

\subsection{Minimal physical motivation}
Although trained via supervised labels, $\mathcal{F}$ is not used as a classifier in this work.
Instead, it functions as a morphology-sensitive measurement map on normalized time--frequency inputs.
Interferometric glitches arise from mechanically mediated elastic disturbances within constrained assemblies, inducing structured time--frequency organization shaped by dispersion, confinement, and mode coupling.
This training induces a latent geometry that can be probed under a strict frozen, zero-shot protocol in physically distinct systems.

\section{Preprocessing and Statistical Scoring Pipeline}
\label{sec:supp_pipeline}

This section documents the fixed preprocessing and statistical scoring used to generate the anomaly score, tail statistics, and Health Index, without expanding the main Methods.

\subsection{Signal resampling and windowing}
All datasets are mapped to a common sampling rate $f_s=4096~\mathrm{Hz}$ using anti-aliasing resampling.
Signals are segmented with $N_{\mathrm{win}}=256$ samples and hop $N_{\mathrm{hop}}=128$ samples.
The choice $f_s=4096\,\mathrm{Hz}$ fixes a common discrete time--frequency grid for all domains and provides adequate resolution for short elastic transients; it is used uniformly across datasets and not tuned per target domain. We emphasize that changing this grid alters the \emph{measurement resolution} of the instrument, rather than constituting any form of target-domain adaptation.

\subsection{Time--frequency representation}
For each window we compute an STFT with Hann window, $N_{\mathrm{fft}}=256$, and \texttt{center=False}.
We form a log-amplitude spectrogram
\begin{equation}
X=\log\!\left(1+\left|\mathrm{STFT}\right|\right).
\end{equation}
We apply per-window standardization (zero mean and unit variance per window) to suppress absolute scale while preserving relative time--frequency organization. Spectrogram windows are then mapped to the encoder input format (fixed spatial resolution and channels) using a deterministic procedure implemented in the accompanying code.

\subsection{Frozen embedding}
Each processed window is mapped by the frozen operator:
\begin{equation}
\mathcal{F}:\; X\in\mathbb{R}^{M\times N}\mapsto z\in\mathbb{R}^{1280},
\end{equation}
using the EfficientNet-B0 feature stack plus global average pooling.
No retraining or adaptation is performed.
All thresholds, tail statistics, and confidence intervals reported in the manuscript
are defined consistently on the distance-form score $\mathcal{S}$ in
Eq.~(\ref{eq:maha_app}); the quadratic form is not used for thresholding or aggregation.

\subsection{Nominal baseline and Mahalanobis score}
A nominal reference set $\mathcal{P}_0$ is constructed from early-life (IMS) or known-normal data (static benchmarks).
We estimate the mean $\mu_0$ and a Ledoit--Wolf shrinkage covariance $\Sigma_{\mathrm{LW}}$ on $\mathcal{P}_0$,
and define the (distance-form) Mahalanobis score:
\begin{equation}
\mathcal{S}(z)=\sqrt{(z-\mu_0)^{\top}\Sigma_{\mathrm{LW}}^{-1}(z-\mu_0)}.
\label{eq:maha_app}
\end{equation}
All thresholds and tail statistics are defined on $\mathcal{S}$.

\subsection{Fixed threshold and tail enrichment}
We use a fixed nominal threshold
\begin{equation}
\tau = Q_{0.999}\!\left(\mathcal{S} \mid \mathcal{P}_0\right),
\end{equation}
corresponding to a nominal false-alarm probability $1-q=10^{-3}$.
Tail enrichment is defined as
\begin{equation}
\Lambda_{\mathrm{tail}}=
\frac{
\mathbb{P}\!\left(\mathcal{S}>\tau \mid \mathrm{abnormal}\right)
}{
\mathbb{P}\!\left(\mathcal{S}>\tau \mid \mathrm{nominal}\right)
}.
\end{equation}
\paragraph{Intellectual property.}
Portions of the methodology underlying the present work are the subject of a
separate patent application. The scientific results and conclusions reported
here are independent of any proprietary implementation.
\bibliographystyle{apsrev4-2}
\bibliography{references}
\end{document}
